# Supplementary material for: A unified state diagram for the yielding transition of soft colloids
Source: arXiv:2212.08863 source file (2022-12-17)
Supplement: Supplementary file 1 [file 221216_SI_black_version_nonumbers.pdf]

# SUPPLEMENTARY INFORMATION TO "A UNIFIED STATE DIAGRAM FOR THE YIELDING TRANSITION OF SOFT COLLOIDS"

Stefano Aime*,[1,2] Domenico Truzzolillo,[1] David J. Pine,[3] Laurence Ramos,[1] and Luca Cipelletti*[1,4]

[1] *Laboratoire Charles Coulomb (L2C), Université Montpellier, CNRS, Montpellier, France*

[2] *Present address: ESPCI, Paris, France**

[3] *New York University*

[4] *Institut Universitaire de France*†

## TABLE OF CONTENTS

Supplementary information to "A unified state diagram for the yielding transition of soft colloids" .......... 1

Table of contents .......... 1

I. Experimental setups .......... 2

II. Additional experimental data and fit parameters .......... 5

II.a Experimental and fit parameters .......... 5

II.b Strain amplitude dependence of the viscoelastic moduli .......... 6

II.c Dynamics at rest or in the $\gamma_0 \to 0$ limit .......... 7

II.d Scattering vector dependence of the dynamics and of the model parameters .......... 8

II.e Impact of the oscillatory frequency (samples M2s and M40s) .......... 13

III. Numerical model .......... 14

IV. Spatial heterogeneity of the dynamics and shear bands .......... 17

References .......... 20

# I. EXPERIMENTAL SETUPS

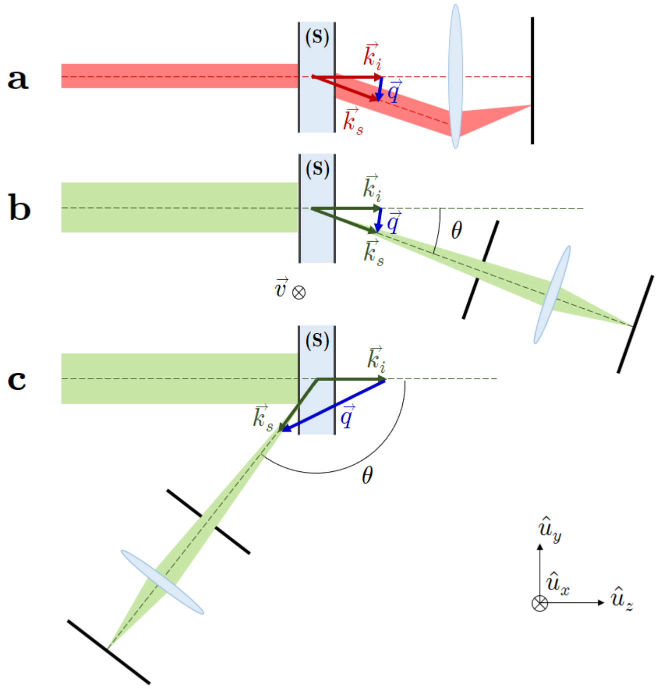


**Figure SI1: Sketch of dynamic light scattering (DLS [1]) setups.**

a) Far-field light scattering setup used for sample M40s: the detector is in the focal plane of the lens. b) Small-angle Photon Correlation Imaging (PCI) setup used for sample M2s: the lens images the sample S onto the detector; only light scattered at angles near to the scattering angle $\theta$ contributes to the image formation. c) Wide-angle PCI setup used for N samples: same imaging geometry as in b), but for a larger scattering angle. In all sketches, $\overrightarrow{\boldsymbol{u_x}}, \overrightarrow{\boldsymbol{u_y}}, \overrightarrow{\boldsymbol{u_z}}$ denote velocity, vorticity and gradient directions, respectively. $\overrightarrow{\boldsymbol{k_\iota}}, \overrightarrow{\boldsymbol{k_s}}$ and $\overrightarrow{\boldsymbol{q}}$ denote the incoming and scattered wave vectors and the scattering vector, respectively. The shear cell is not shown for clarity.

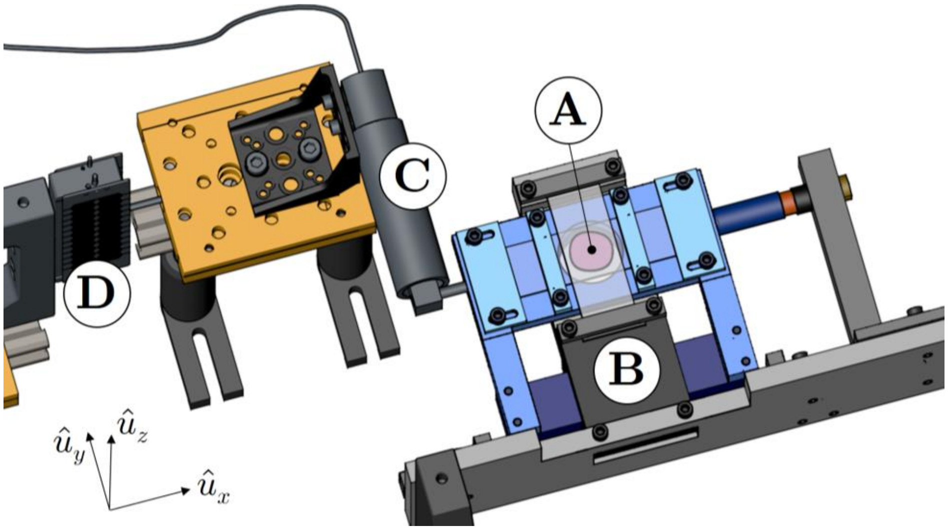


**Figure SI2: Sketch of the custom shear cell for the DLS setups.**

A) Sample, confined between two transparent parallel plates; B) shear cell, mounted on an air bearing stage [2] C) stress sensor (Model LC601, from Omega Engineering) D) strain piezoelectric actuator (P602, from Physik Instrumente). $\overrightarrow{\boldsymbol{u_x}}, \overrightarrow{\boldsymbol{u_y}}, \overrightarrow{\boldsymbol{u_z}}$ denote velocity, vorticity and gradient directions, respectively.

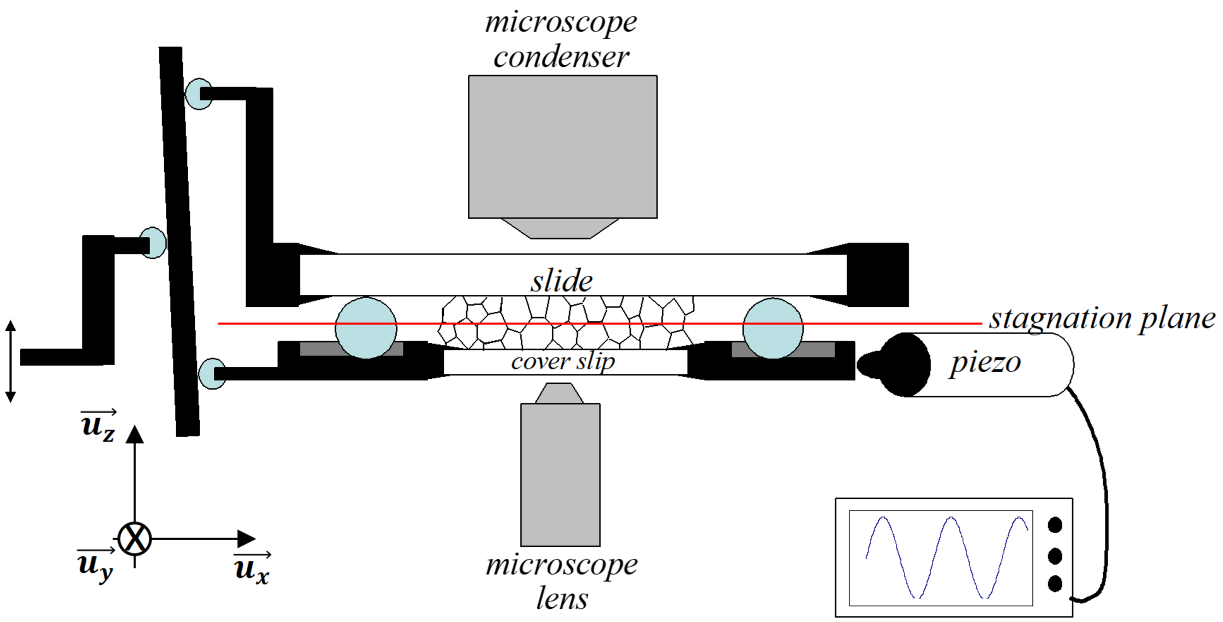


**Figure SI3: Sketch of the custom shear cell for the emulsion samples.**

The sample is imaged in the stagnation plane (indicated by the red line), which is at rest in the laboratory frame. $\vec{u_x}, \vec{u_y}, \vec{u_z}$ denote velocity, vorticity and gradient directions, respectively. Adapted from [3]. Data collected with this setup are analyzed using Digital Fourier Microscopy [4].

# II. ADDITIONAL EXPERIMENTAL DATA AND FIT PARAMETERS

## II.a Experimental and fit parameters

| Sample | $\gamma_{min}$ | $\gamma_{max}$ | $\nu$ | $\beta_0$ | $(1/\tau_0)/s^{-1}$ | $\beta_s$ | $\beta_f$ | $\omega\Gamma_s/s^{-1}$ |
|---|---|---|---|---|---|---|---|---|
| M2s | 0.1% | 62% | 0.6 | 1.5 | $2.5 \times 10^{-5}$ | 1.3 | 0.33 | $2 \times 10^{-5}$ |
| M40s | 2.8% | 69% | 0.6 | 1.5 | $2.5 \times 10^{-5}$ | 1.6 | 0.44 | $2 \times 10^{-5}$ |
| N41% | 0.01% | 72% | 0.75 | 1.2 | $1.4 \times 10^{-4}$ | 1.4 | 0.36 | $1 \times 10^{-4}$ |
| N41%Aged | 0.01% | 8.6% | 0.75 | 1.2 | $1.4 \times 10^{-4}$ | 1.2 | 0.90 | $1 \times 10^{-4}$ |
| N45% | 1% | 25% | 0.7 | 1.9 | $1.2 \times 10^{-4}$ | 1.9 | 0.88 | $1.1 \times 10^{-4}$ |
| E65% | 0.4% | 6.4% | 0.6 | | | 1.5 | 0.34 | $1.6 \times 10^{-3}$ |
| E70% | 1.2% | 6.4% | 0.65 | | | 1.0 | 0.40 | $1.3 \times 10^{-4}$ |
| E74% | 4.8% | 12% | 0.65 | | | 1.4 | 0.32 | $6.1 \times 10^{-4}$ |
| E88% | 5.4% | 20% | 0.7 | | | 1.7 | 0.29 | $6.6 \times 10^{-4}$ |

**Table SI1: Experimental and fit parameters for the probed samples.**

Minimum ($\gamma_{min}$) and maximum ($\gamma_{max}$) applied strain deformations, terminal slopes $\nu$ of $G''(\gamma_0)$ defined in Fig. 1a of the main text, spontaneous relaxation rate $1/\tau_0$ and stretching exponents $\beta_0$, $\beta_s$, $\beta_f$ of the fits to correlation functions (see main text for the definitions). The relaxation rates shown here are measured at representative scattering vectors $q$=5 $\mu m^{-1}$, 30 $\mu m^{-1}$ and 9 $\mu m^{-1}$ for M, N and E samples, respectively. For the M and N samples, $\beta_0$ and $\tau_0$ are measured at rest. For the E samples, no correlation functions at rest are available, but $\beta_s$ and $\omega\Gamma_s$ are obtained, as for the other samples shown in the table, in the low strain regime, where these parameters are essentially strain-independent and representative of the behavior at rest. For sample E70%, the decay of the correlation functions in the $\gamma_0 \rightarrow 0$ limit is modest, making it difficult to determine unambiguously $\beta_s$, whose value was thus set to unity.

Shear protocol: All samples were presheared before each measurement at a given $\gamma_0$, using oscillatory shear at the same $\omega$ as for the subsequent measurement. Samples E were presheared for several minutes at a high strain, typically 250–300%. The strain amplitude was then reduced to the target value and at least 300 cycles were imposed at the target $\gamma_0$ before starting the image acquisition, which lasted 1000 cycles or more. Samples M and N were presheared at the largest $\gamma_0$ to be tested. The preshear lasted 500 oscillations for sample M40s, 5000 for all other M and N samples. After presehar, shear at each amplitude had 2500 oscillations (sample M40s) or 50000 oscillations (all other M and N samples). We changed the order at which the various $\gamma_0$ values were tested (including by varying $\gamma_0$ non-monotonically), finding that our results did not depend on the specific sequence of tested strain amplitudes.

II.b Strain amplitude dependence of the viscoelastic moduli

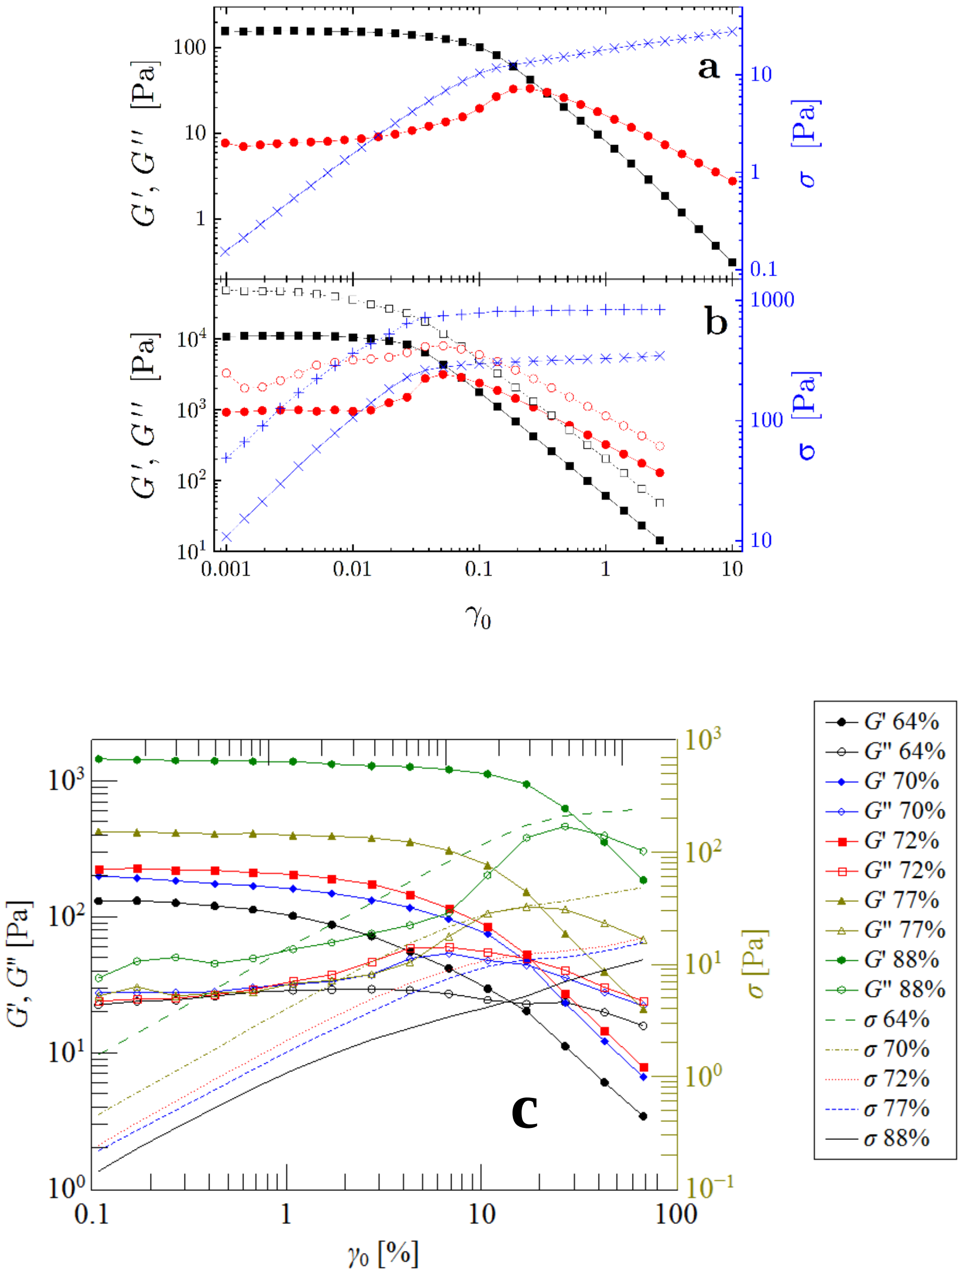


**Figure SI4: Rheology data for all samples.**

Dependence of the viscoelastic moduli *G*' and *G*" and of the shear stress $\sigma$ on shear strain. a: microgels (same data as in Fig. 1 of the main text); b: nanoparticle samples, $\varphi$ = 43.5% (solid symbols and crosses) and 46% (open symbols and pluses); c: emulsions [3]. In panels a and b, squares, circles and crosses or pluses correspond to *G*', *G*", and $\sigma$, respectively. Data in a were collected in the custom shear cell of Fig. SI2. All other data were obtained using a commercial rheometer. For the N and E samples, the volume fraction is slightly different from that of the corresponding samples used for light scattering and microscopy, which entails no significant difference in the rheological properties with respect to those shown here.

## II.c Dynamics at rest or in the $\gamma_0 \rightarrow 0$ limit

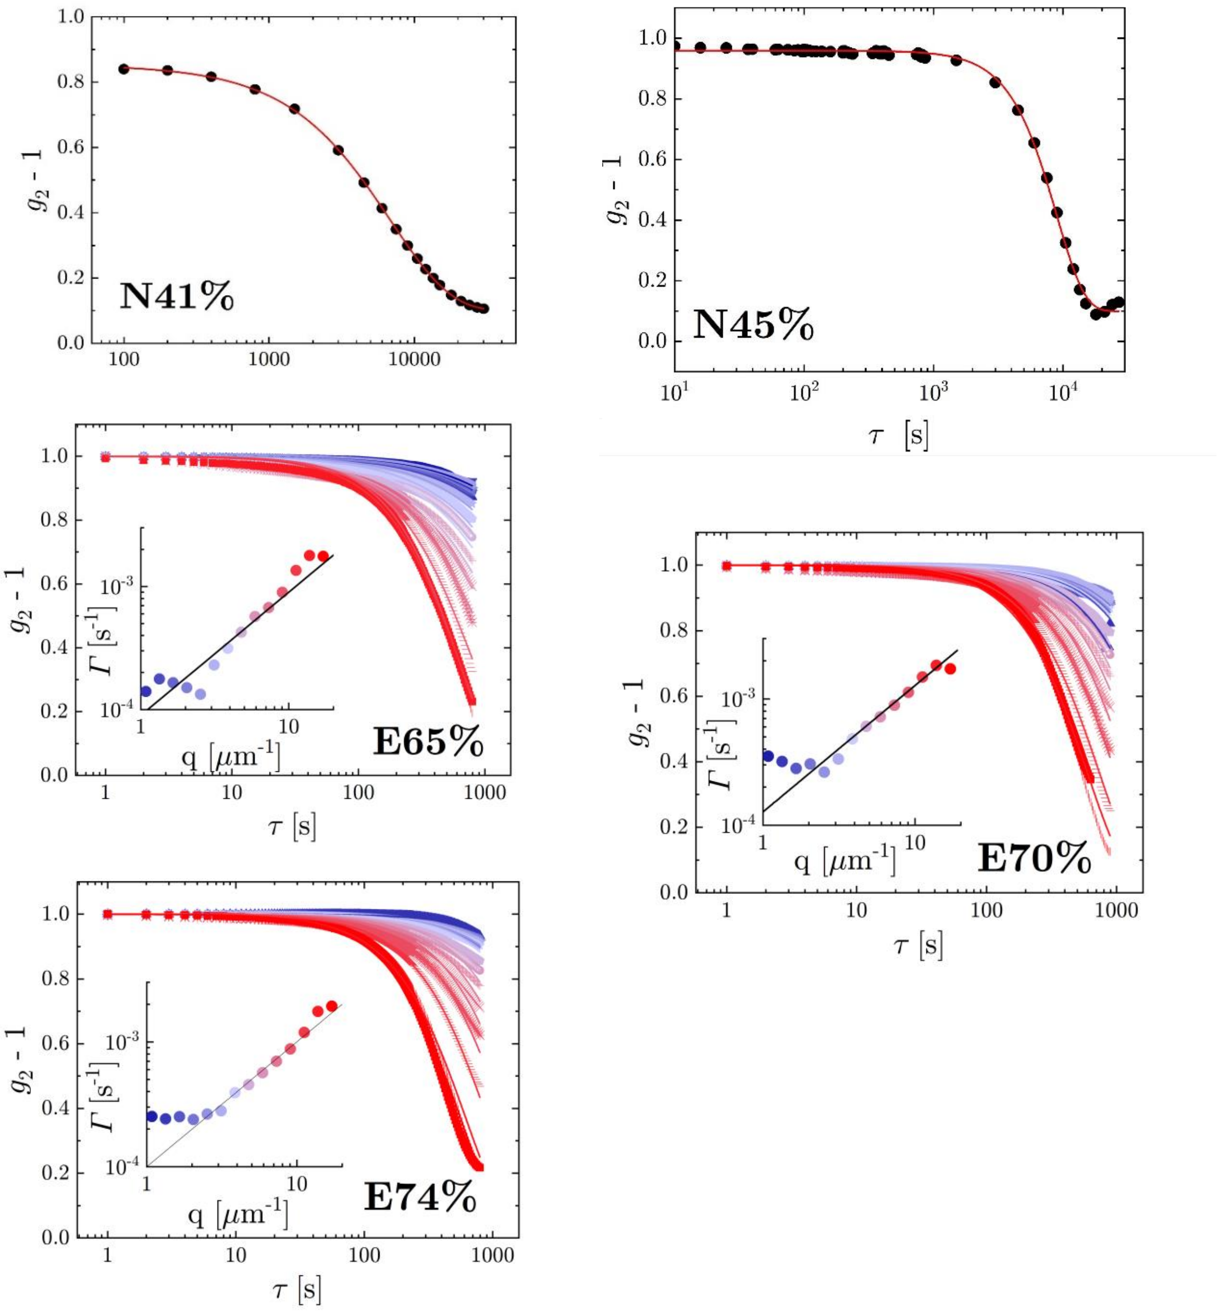


**Figure SI5: Dynamics at rest or in the $\gamma_0 \rightarrow 0$ limit for N and E samples.**

Intensity correlation functions for various N and E samples. For N samples, data are taken at rest. For E samples, data are taken in the low-strain regime where the dynamics are essentially independent of the applied strain: $\gamma_0$ = 1.18%, 0.36% and 3.85% for E65, E70, and E74, respectively. For the E samples, in the insets the line shows that the relaxation rate scales as $q$, indicative of ballistic dynamics. Deviations from ballistic behavior are observed only at very low $q$, most likely because the decay of $g_2$-1 is too small for the fit to capture reliably the relaxation time.

II.d Scattering vector dependence of the dynamics and of the model parameters

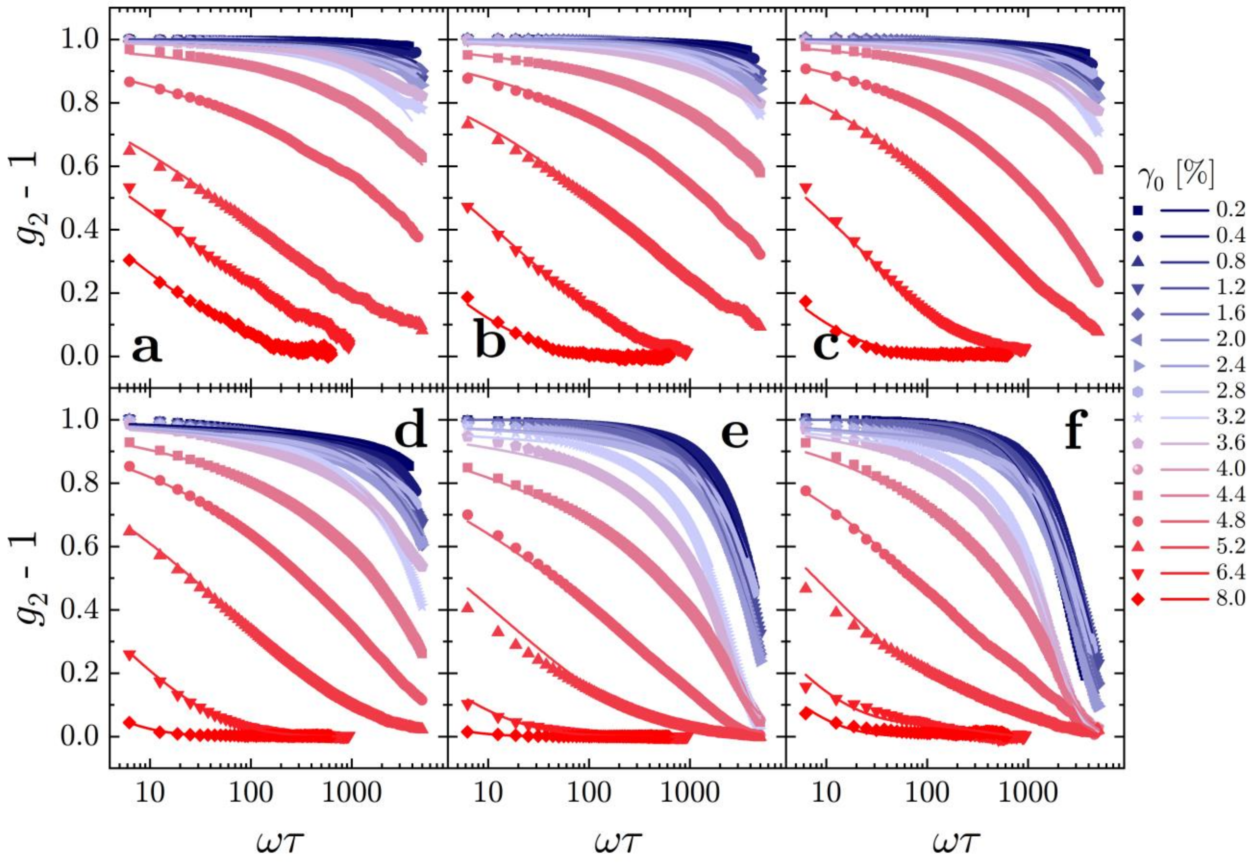


**Figure SI6: Scattering vector dependence of correlation functions, sample E64.**

Intensity correlation functions for sample E64%, for various imposed strain amplitudes as shown by the labels. Values of the scattering vector $q$: 0.7 µm$^{-1}$ (a), 1.3 µm$^{-1}$ (b), 2.5 µm$^{-1}$ (c), 4.8 µm$^{-1}$ (d), 9 µm$^{-1}$ (e), 14 µm$^{-1}$ (f).

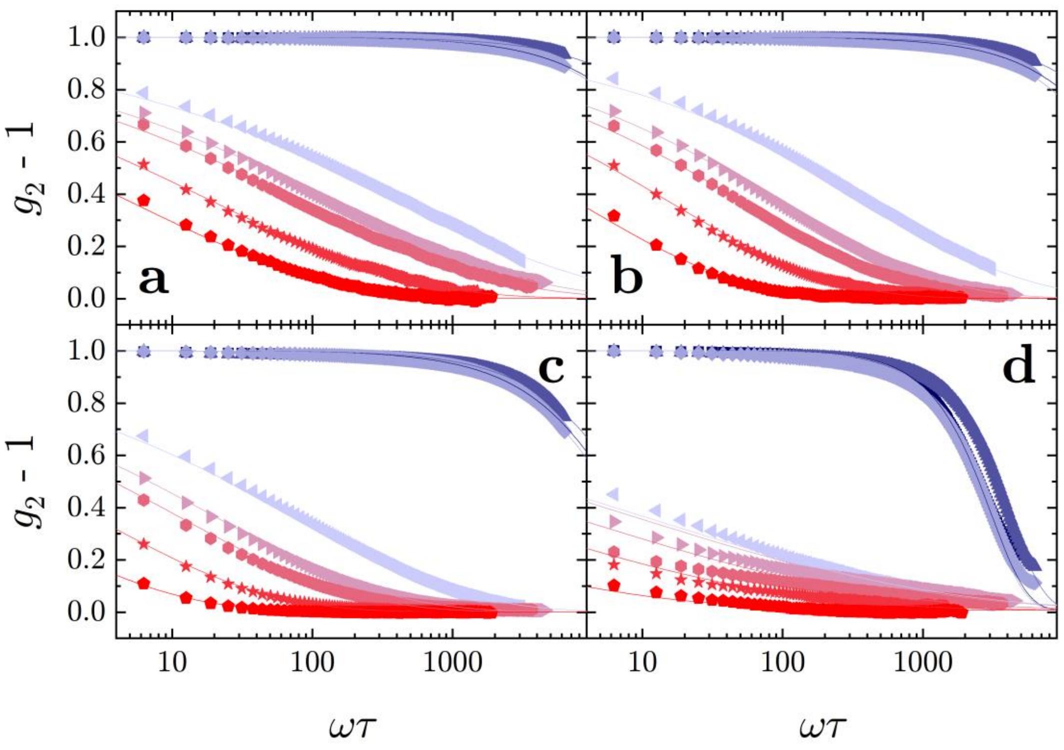


**Figure SI7: Scattering vector dependence of correlation functions, sample E74.**

Intensity correlation functions for sample E74% (same sample and color code as in Fig. 2c of the main text, which shows data at $q$ = 9 µm$^{-1}$). Values of the scattering vector $q$: 1.3 µm$^{-1}$ (a), 2.5 µm$^{-1}$ (b), 4.8 µm$^{-1}$ (c), 14 µm$^{-1}$ (d).

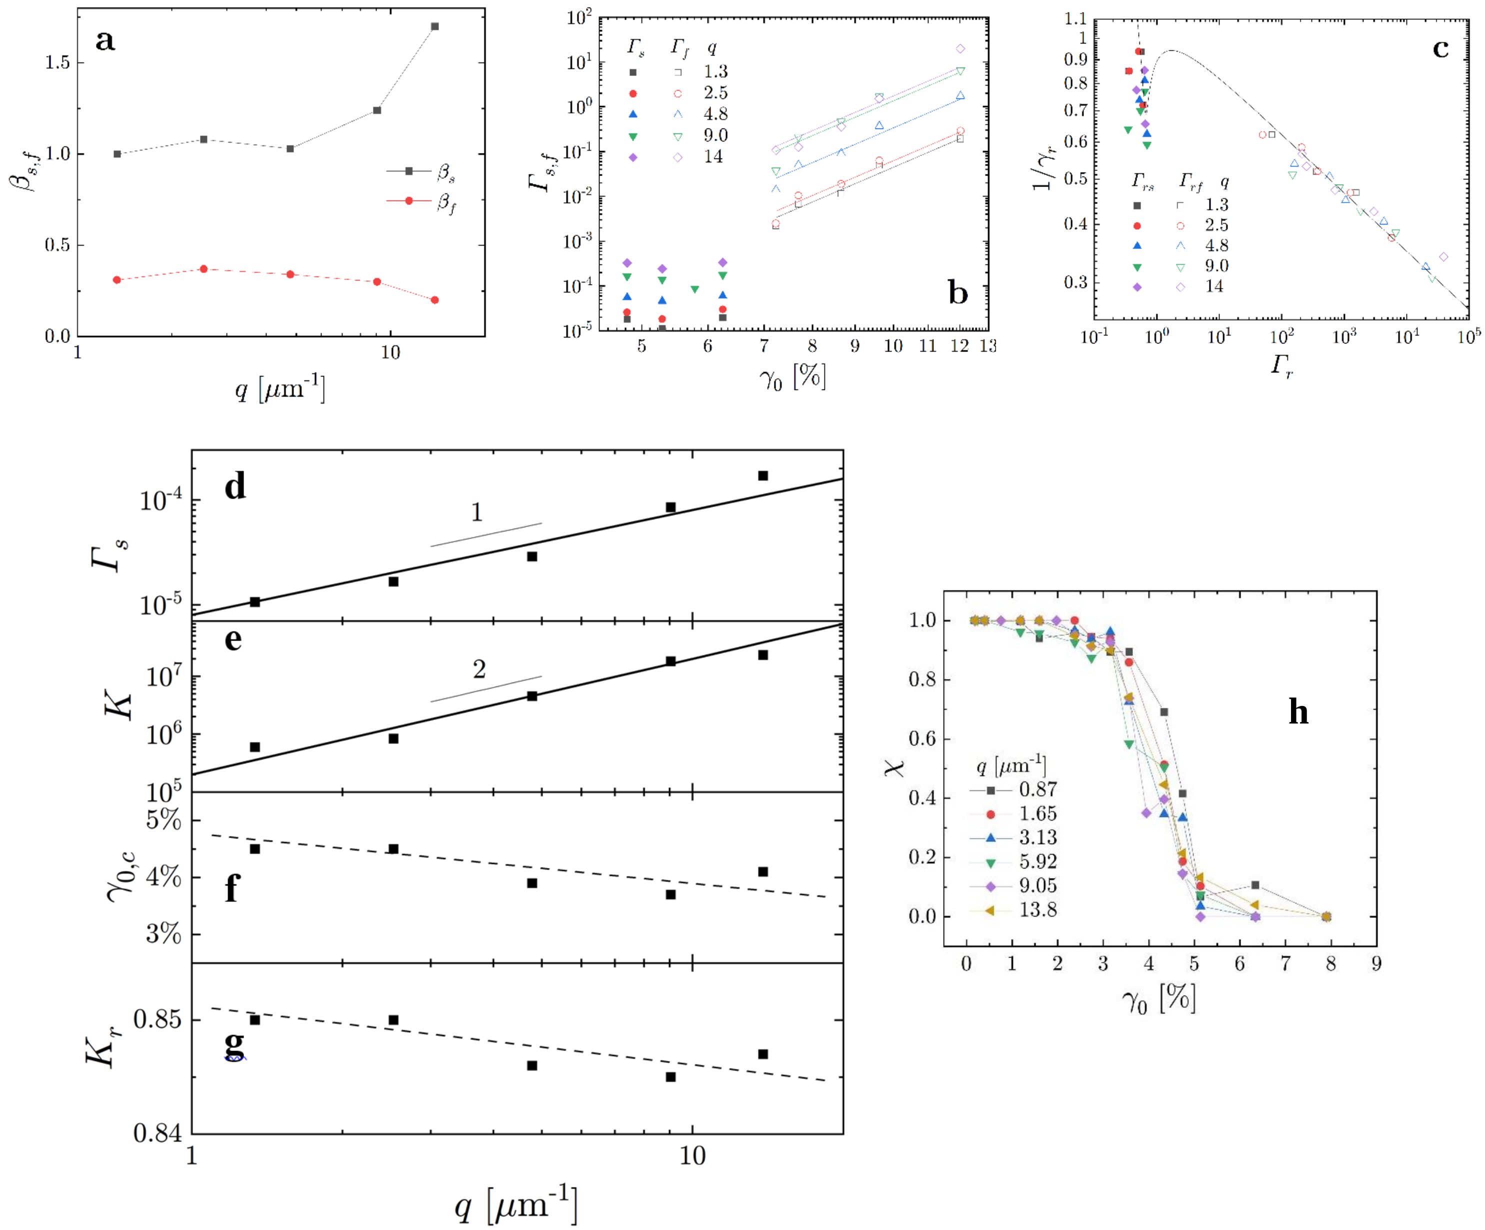


**Figure SI8: Scattering vector dependence of various model and fit parameters.**

Scattering vector dependence of various model and fit parameters for representative E samples. a-g: sample E74%; h: sample E64%.

a): $q$ dependence of the stretching exponent $\beta_f$ for the fast decay and compressing exponent $\beta_s$ for the slow decay. $\beta_f$ depends only mildly on $q$. At low $q$, $\beta_s$ approaches unity, most likely because the limited decay of $g_2$-1 prevents the shape of the correlation function to be characterized precisely (see Fig. SI7a-c).

b): $q$ and strain amplitude dependence of the relaxation rates of the fast and slow modes. In the large strain regime, $\Gamma_f$ grows as a power-law of $\gamma_0$, with an exponent $n$ independent of $q$, as indicated by the parallel lines in the double logarithmic plot.

c): state diagram in the spirit of Fig. 4 of the main text, but obtained from data at different $q$ vectors. All data collapse on the same curve, demonstrating that the model is robust with respect to the choice of $q$.
d): relaxation rate of the spontaneous dynamics, obtained by extrapolating data under shear to the $\gamma_0 \rightarrow 0$ limit. The relaxation rate increases as $q$, indicative of ballistic dynamics.
e): the model parameter $K$ (akin to temperature $T$ in Van der Waal's equation of state for real gases) grows as $q^2$. At large strain, Eqs. 2a-2b of the main text show that $\Gamma \sim \Gamma_f \sim K/\gamma_0^{-n}$. Thus, the $K \sim q^2$ scaling shown here implies $\Gamma \sim \Gamma_f \sim q^2$, i.e. that the dynamics at large strain are diffusive (see also Fig SI9).
f): the yield strain $\gamma_{0,c}$ extracted by fitting the model to the microscopic dynamics exhibits only a mild dependence on the scattering vector $q$.
g): the model parameter $K$ expressed in reduced units (i.e. $K$ normalized by its value $K_c$ at the critical point) is nearly independent of the $q$ vector.
h): The normalized amplitude of the slow mode, $\chi$, depends only very weakly on the $q$ vector at which the microscopic dynamics are measured. This is consistent with the notion that the yield strain inferred from the microscopic dynamics is nearly insensitive to $q$, as shown in f. Furthermore, the data in h show that the width of the coexistence region is nearly independent of $q$. Because in the model the width of the coexistence region is mainly controlled by the amount of disorder, these data indicate that the latter is essentially insensitive to the choice of $q$.

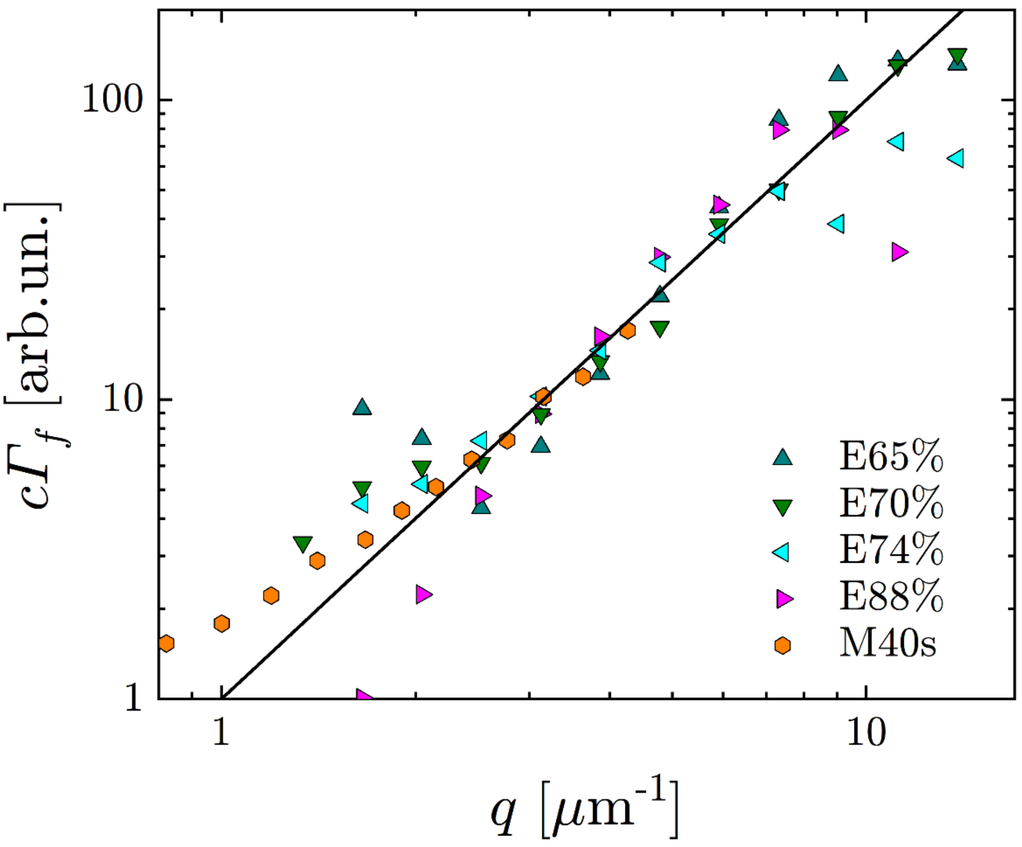


**Figure SI9: Diffusive dynamics in the fluidized regime.**

Symbols: relaxation rates measured in the fully fluidized regime (strain amplitudes: $\gamma_0$=5% for E65% and E70%, $\gamma_0$=7% for E74%, $\gamma_0$=16% for E88%, $\gamma_0$=50% for M40s). Datasets have been rescaled vertically by multiplying them by a constant *c*, to highlight the overall $\boldsymbol{\Gamma_f \propto q^2}$ behavior indicative of diffusive dynamics (solid line).

II.e Impact of the oscillatory frequency (samples M2s and M40s)

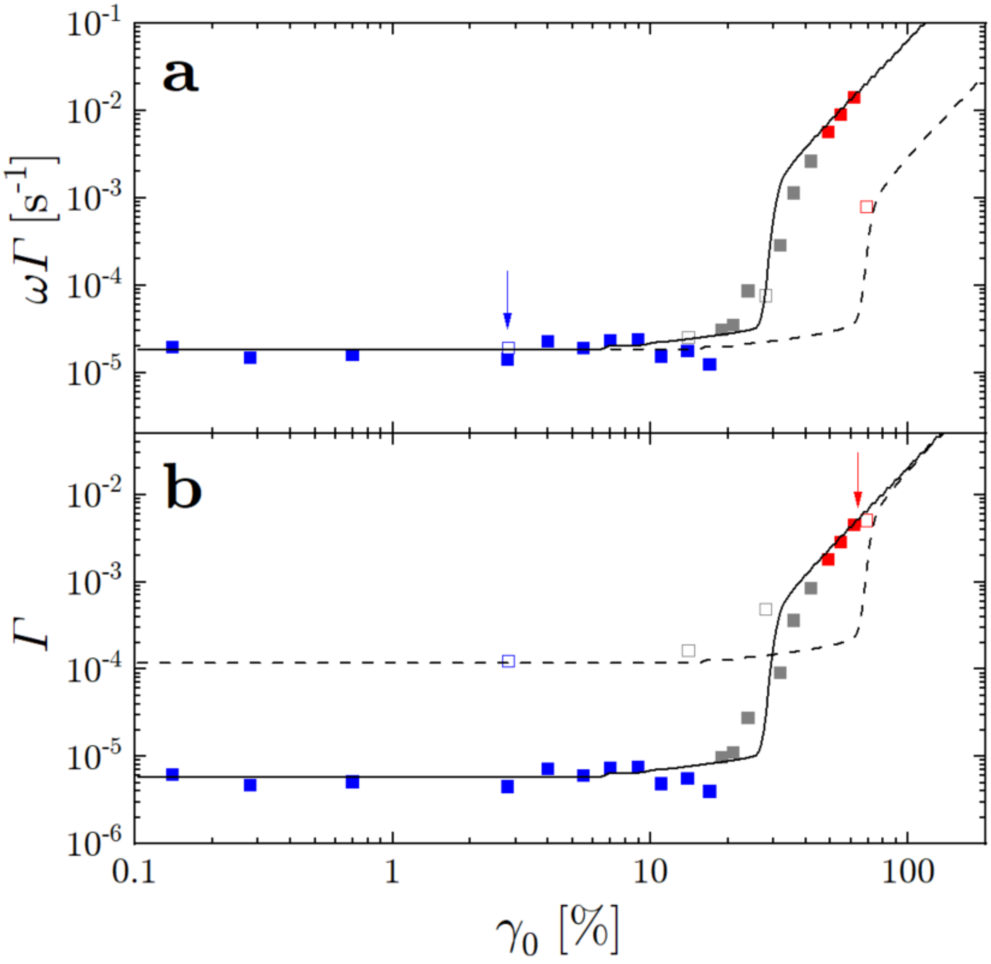


**Figure SI10: Impact of oscillatory frequency.**

Relaxation rate (a) and normalized relaxation rate (b) as a function of strain amplitude, for dense microgel suspensions measured at two different oscillatory frequencies, corresponding to a period of 2s (full symbols, sample M2s), and 40s (empty symbols, sample M40s), respectively. Blue, red and gray symbols refer to compressed (solid-like), stretched (fluid-like), and two-step (coexistence) relaxations, respectively. Arrows highlight the collapse of solid-like relaxations when using physical units (panel a)), and of liquid-like relaxations when using relaxation rates normalized by the angular frequency of the imposed oscillatory shear (panel b)). Lines: numerical solutions reproducing the observed behavior with shared model parameters $\Gamma_0 = 2\ 10^{-5} s^{-1}$ and $K = 4\ 10^{-3}$. The average coupling constants are $\bar{\bar{\alpha}} = 9\ 10^{-8}$ for M2s (solid line) and $\bar{\alpha} = 1.6\ 10^{-6}$ for M40s (dashed line).

# III. NUMERICAL MODEL

| | Unit | M2s | M40s | N41% | N41%Aged | N45% | E65% | E70% | E74% | E88% |
|---|---|---|---|---|---|---|---|---|---|---|
| $1/\tau_0$ | **1/s** | **$2\ 10^{-5}$** | **$2\ 10^{-5}$** | **$10^{-4}$** | **$10^{-4}$** | **$1.1\ 10^{-4}$** | **$1.6\ 10^{-3}$** | **$1.3\ 10^{-4}$** | **$6.1\ 10^{-4}$** | **$6.6\ 10^{-4}$** |
| $1/\omega\tau_0$ | - | $6.4\ 10^{-6}$ | $1.3\ 10^{-4}$ | $3\ 10^{-5}$ | $3\ 10^{-5}$ | $3.5\ 10^{-5}$ | $3\ 10^{-4}$ | $2\ 10^{-5}$ | $10^{-4}$ | $1.1\ 10^{-4}$ |
| $\omega$ | rad/s | 3.14 | 0.157 | 3.14 | 3.14 | 3.14 | 6.28 | 6.28 | 6.28 | 6.28 |
| $\bar{\alpha}$ | **-** | **$9\ 10^{-8}$** | **$1.6\ 10^{-6}$** | **$1.4\ 10^{-6}$** | **$8\ 10^{-3}$** | **$1.1\ 10^{-3}$** | **$8.8\ 10^{5}$** | **$2\ 10^{4}$** | **$7\ 10^{3}$** | **$4.9\ 10^{2}$** |
| $\sigma_\alpha^2$ | **-** | **$8.9\ 10^{-16}$** | **$1.28\ 10^{-12}$** | **$4.9\ 10^{-13}$** | **$3.2\ 10^{-6}$** | **$9.68\ 10^{-8}$** | **$2.71\ 10^{11}$** | **$8\ 10^{5}$** | **$2.94\ 10^{5}$** | **48** |
| $n$ | **-** | **3** | **3** | **1** | **3** | **3** | **8** | **8** | **8** | **8** |
| $K$ | **-** | **$4\ 10^{-3}$** | **$4\ 10^{-3}$** | **$1.3\ 10^{-2}$** | **62** | **8** | **$10^{9}$** | **$2.4\ 10^{8}$** | **$1.8\ 10^{7}$** | **$1.1\ 10^{6}$** |
| $\omega\Gamma_c$ | rad/s | $6\ 10^{-5}$ | $6\ 10^{-5}$ | $3\ 10^{-4}$ | $3\ 10^{-4}$ | $3\ 10^{-4}$ | $5\ 10^{-3}$ | $4\ 10^{-4}$ | $1.8\ 10^{-3}$ | $2\ 10^{-3}$ |
| $\Gamma_c$ | - | $1.9\ 10^{-5}$ | $4\ 10^{-4}$ | $9\ 10^{-5}$ | $9\ 10^{-5}$ | $1.1\ 10^{-4}$ | $8\ 10^{-4}$ | $6\ 10^{-6}$ | $3\ 10^{-4}$ | $3\ 10^{-4}$ |
| $K_c$ | - | $4.2\ 10^{-3}$ | $4\ 10^{-3}$ | $1.3\ 10^{-2}$ | 72 | 9.3 | $10^{9}$ | $2.9\ 10^{-3}$ | $2.1\ 10^{7}$ | $1.4\ 10^{6}$ |
| $\gamma_{0,c}$ | - | 0.23 | 0.65 | 0.027 | 0.015 | 0.031 | 0.035 | 0.03 | 0.05 | 0.07 |
| $K_r$ | - | 0.89 | 0.98 | 0.97 | 0.85 | 0.86 | 0.99 | 0.84 | 0.85 | 0.84 |
| $g$ | - | 0.11 | 0.02 | 0.03 | 0.15 | 0.14 | 0.01 | 0.16 | 0.15 | 0.16 |
| $d$ | - | 0.11 | 0.5 | 0.25 | 0.05 | 0.08 | 0.35 | 0.002 | 0.006 | 0.0002 |

**Table SI2: Model parameters used to reproduce the experiments.** The fitting parameters are in **red bold** font, parameters fixed by the experiments are in plain black font, and parameters obtained by combining the formers are in blue font. The fitting parameters are obtained by fitting simultaneously, for each sample, $\Gamma_s$, $\Gamma_f$, and $\chi$ as a function of $\gamma_0$, over the whole range of probed strain amplitudes, see e.g. Figs. 2d-2f of the main text.

The parameters listed in the table above have the following meaning:

| | |
|---|---|
| $1/\tau_0$ | Spontaneous relaxation rate (in physical units) |
| $1/\omega\tau_0$ | Normalized spontaneous relaxation rate. |
| $\omega$ | Angular frequency of the imposed oscillatory strain. |
| $\bar{\alpha}, \sigma_\alpha^2$ | Average value and variance of the distribution of coupling constant for the dynamics of neighboring sites. |
| $n$ | Exponent ruling the strain dependence of the fast mode at large strain amplitude, where $\Gamma_f \sim \gamma_0^n$. |
| $K$ | Model parameter in Eq. (3) of the main text, analogous to temperature $T$ in Van der Waals' gas equation. |
| $\omega\Gamma_c$ | Relaxation rate (in physical units) at the critical point in the mean field model, see the discussion of Eq. (4) in the main text. |
| $\Gamma_c$ | Normalized critical relaxation rate. |
| $K_c$ | Value of the model parameter $K$ at the critical point in the mean field model, see the discussion of Eq. (4) in the main text. |
| $\gamma_{0,c}$ | Value of the applied strain at the critical point in the mean field model, see the discussion of Eq. (4) in the main text. |
| $K_r$ | Model parameter $K$ normalized by its critical value: $K_r = K/K_c$. |
| $g$ | 'Glassiness' of a sample, defined by $g = 1 - K_r$ |
| $d$ | Disorder of the coupling constants for the dynamics: $d = \sigma_\alpha^2/\alpha^2$, with $\sigma_\alpha^2$ the variance of the distribution of the coupling constants |

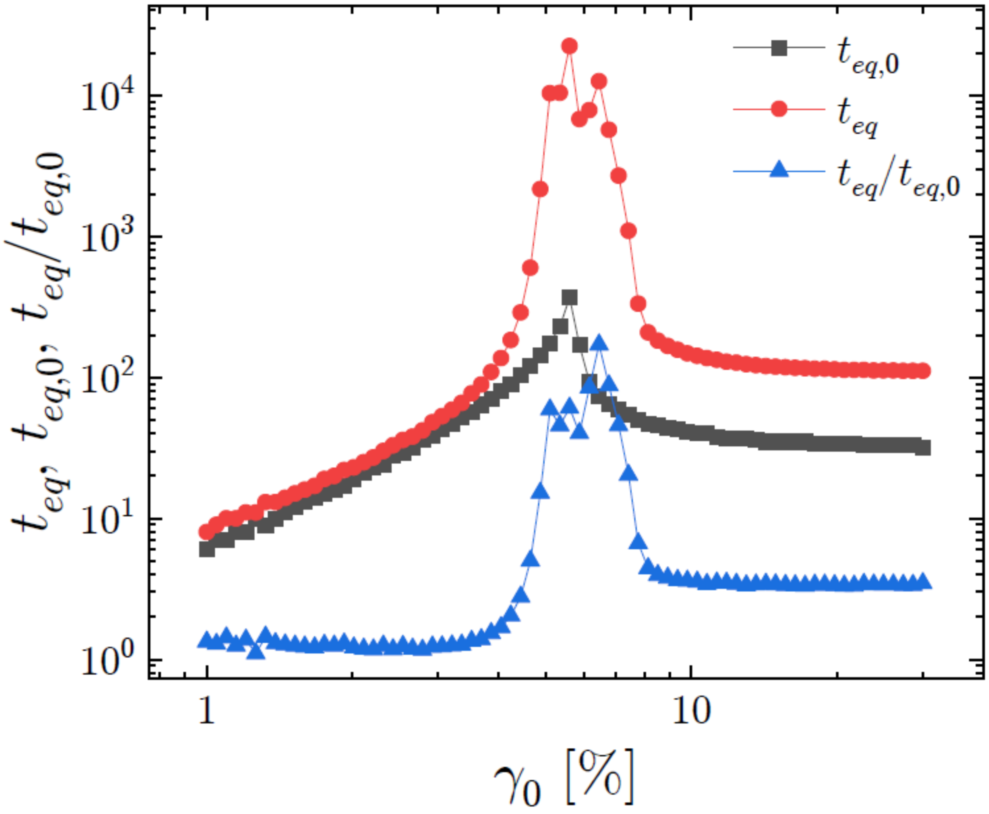


**Figure SI11: Convergence of numerical model: equilibration time.**

Number of iterations needed for the iterative calculation scheme to converge as a function of the strain amplitude, $\gamma_0$, for a model with and without disorder (red circles, $t_{eq}$, and black squares, $t_{eq,0}$, respectively). Blue triangles: $t_{eq}/ t_{eq,0}$ (also shown in Fig. 5f of the main text). The model is implemented on a 2D lattice with 512 x 512 sites. The model parameters correspond to the fit to sample N45% (see Table SI2).

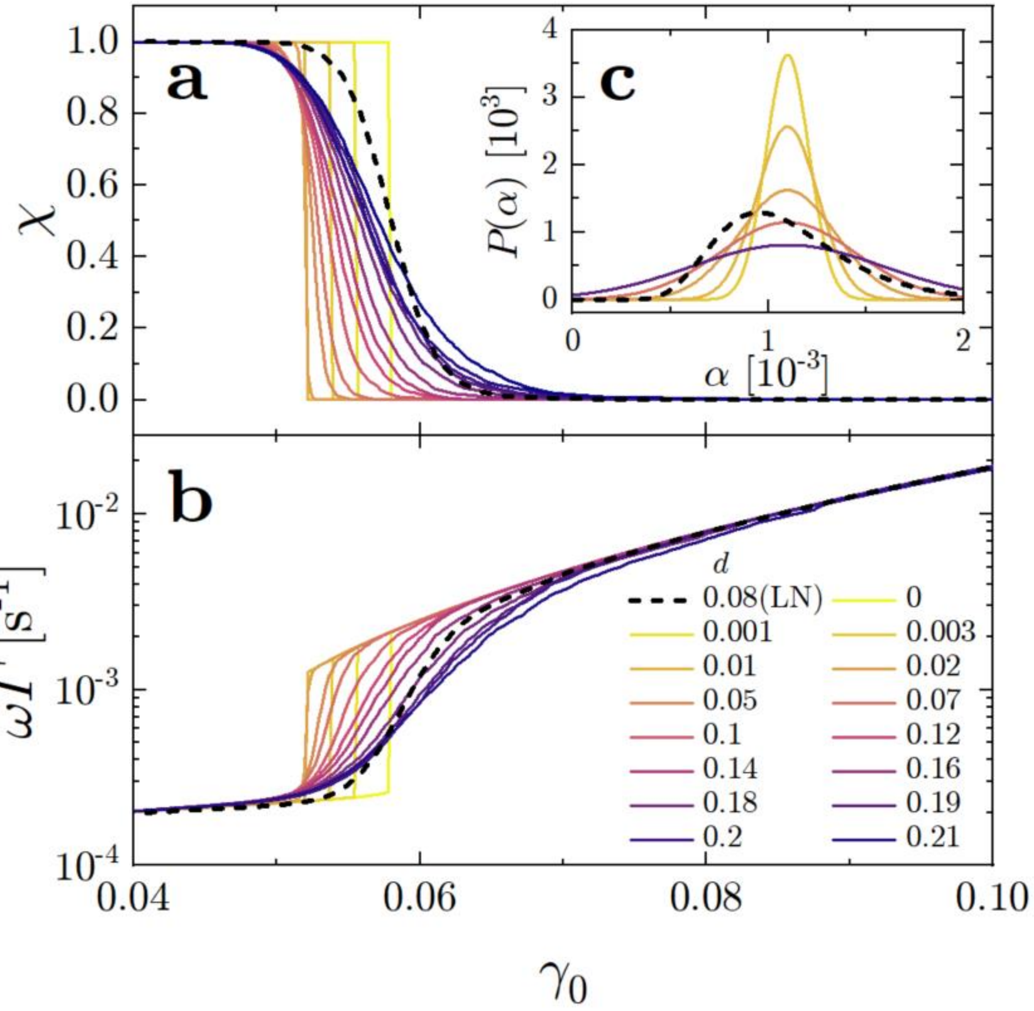


**Figure SI12: Dependence on disorder.**

Changing the nature of the probability distribution function (PDF) of the coupling constants does not change the main features of the transition. Panels a) and b): Order parameter $\chi$ (a) and normalized average relaxation rate $\Gamma$ (b) extracted from the numerical model as a function of strain amplitude, $\gamma_0$, for various PDFs. The model parameters are issued from the fit to N45 (see Table SI2). The coupling constants $\alpha_{i,j}$ are drawn from a Log-Normal PDF (LN, black dashed line), as in the main text, or from Gaussian PDFs, with increasing disorder $d = \sigma_\alpha^2/\bar{\alpha}^2$ from yellow to purple shades, as specified in the legend. The left tails of the Gaussian PDFs are truncated to insure $\alpha_{i,j} \geq 0$. Panel c): representative PDFs used to generate the data in a) and b) (for the sake of clarity, not all the PDFs are shown).

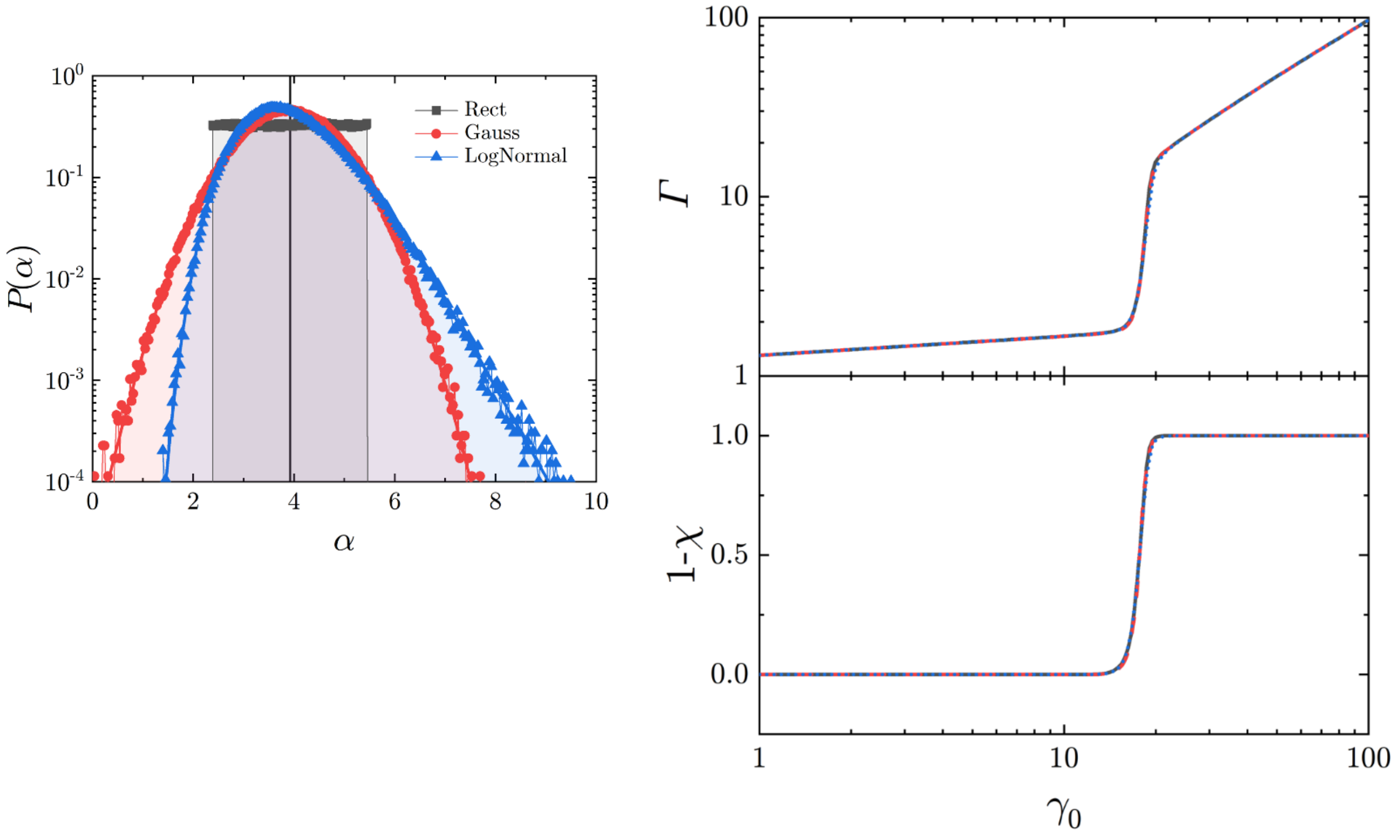


**Figure SI13: Changing the PDF of the coupling constants does not modify the model predictions.**

Left panel: shape of three probability distribution functions (PDF) used to test numerically the impact of the PDF of the coupling constant $\alpha$ on the predictions of the model. Black, red and blue points refer to a rectangular, Gaussian and log-normal PDF, respectively. The left tail of the Gaussian PDF is truncated to insure $\boldsymbol{\alpha_{i,j} \geq 0}$. The right panels show that the shape of the PDF has no impact on the strain amplitude dependence of the relaxation rate (top) or the relative amplitude of the fast mode $\chi$-1 (bottom).

## IV. SPATIAL HETEROGENEITY OF THE DYNAMICS AND SHEAR BANDS

We test in a few samples the spatial heterogeneity of the dynamics and the existence of shear bands.

In the geometry of our experiments, shear bands would develop most likely as layers with different shear deformation organized perpendicularly to the shear gradient direction (the $\overrightarrow{\boldsymbol{u_z}}$ direction in the schemes of Figs. SI1- SI3) and parallel to the shear direction. In the light scattering setups used in this work, the scattered light is collected from the whole thickness of the illuminated sample, with no spatial resolution along the shear gradient direction. It is therefore very difficult to test directly the existence of shear bands. However, we note that if shear bands parallel to the shear direction would exist, the dynamics detected in our space-resolved setup (e.g. the PCI setup of Fig. SI1c) would be spatially homogeneous. Indeed, scattered light exiting from the shear cell and forming the image on the detector would have equally probed all bands, irrespective of the positions in the ($x$,$y$) plane that is imaged.

Figure SI14 shows that this is not the case: instead, in the coexistence region the sample partitions in localized domains of fast and slow dynamics, incompatible with shear bands parallel to the shear direction.

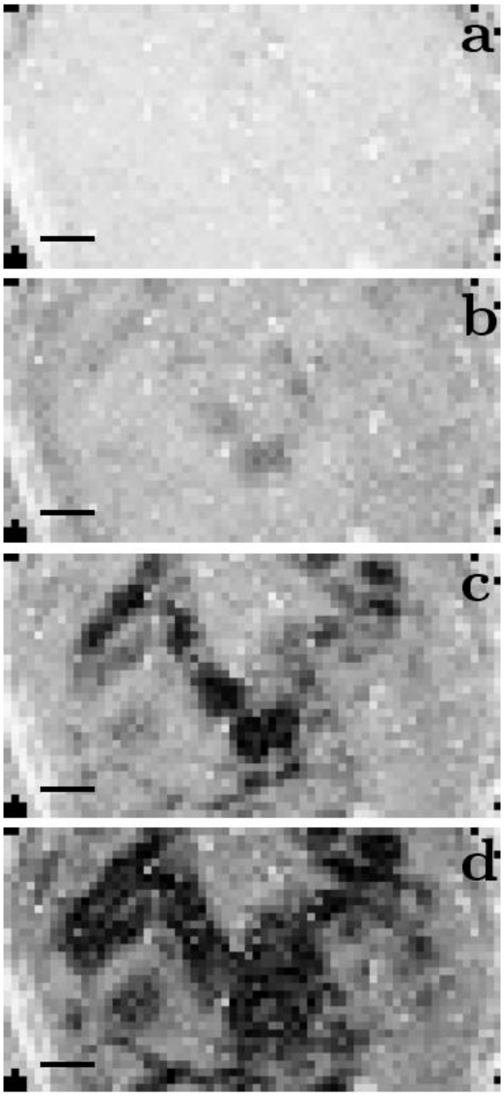


**Figure SI14: Coexistence of fast and slow domains as probed by light scattering**.

Stroboscopic correlation maps for sample N45% in the coexistence region (strain amplitude $\gamma_0$ = 5.7%), for different time delays $\tau/T$ = 32 (a), 128 (b), 512 (c), 1024 (d)). The amount of correlation is represented by a gray scale from black ($g_2$-1=0) to white ($g_2$-1=1). Scale bars: 1mm.

Experiments on emulsions are consistent with this scenario. They probe a thin sample slab (thickness ~ 0.5 μm, smaller than the drop size), parallel to the shear direction. The observation of the coexistence of two relaxation modes under these conditions (see sample E65%, Fig. SI15) rules out the hypothesis that the

observed bimodal relaxation stems from distinct shear bands organized perpendicularly to the shear gradient direction.

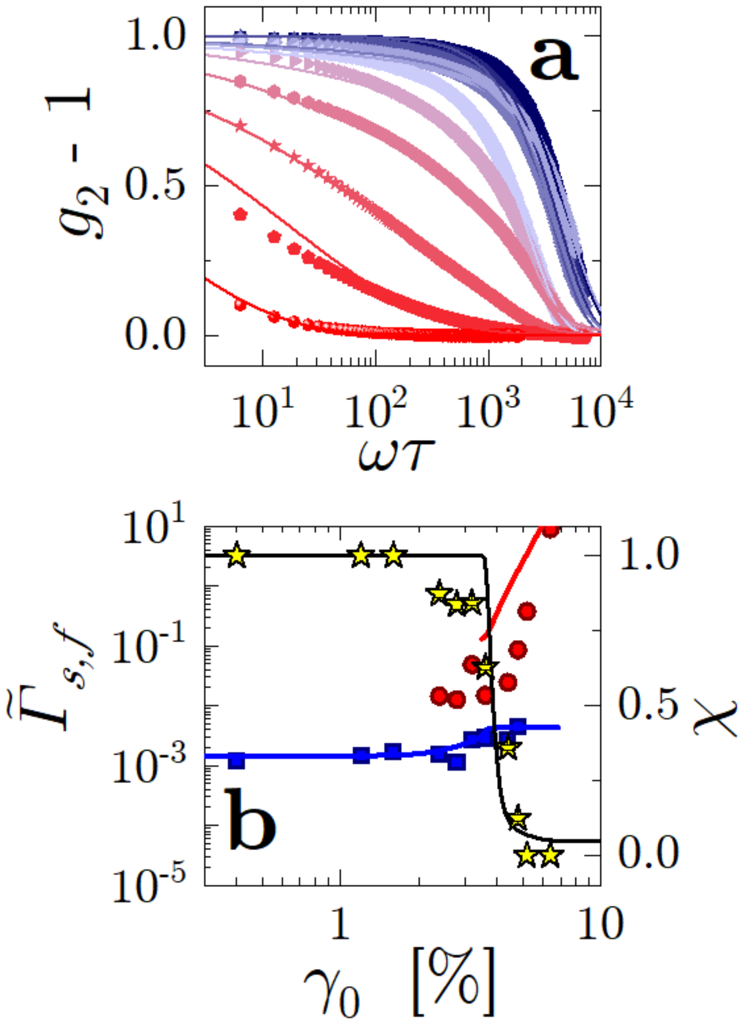


**Figure SI15: Dynamic coexistence in emulsions (sample E65%)**

a) Intensity correlation functions for sample E65%, plotted *vs* the normalized time delay $\omega\tau$, as in Fig. 2 of the main text. Symbols: experimental data. Lines: fits using Eq. 1 of the main text. b) Symbols: fitting parameters. Left axis: normalized relaxation rates for slow and fast modes (blue squares and red circles, respectively). Right axis: relative amplitude $\chi$ of the slow mode (stars). Lines: result of numerical model with parameters reported in Table SI2.

Furthermore, a direct visualization of the regions undergoing fast rearrangements may be obtained by taking the difference between the intensity of microscopy images taken at different times, as shown in Fig. SI16. In this representation, quiescent regions appear uniformly gray, whereas features on the drop size length scale emerge in the rearranged regions. One clearly sees the emergence of localized domains of fast-moving drops, once again incompatible with shear bands parallel to the shear direction.

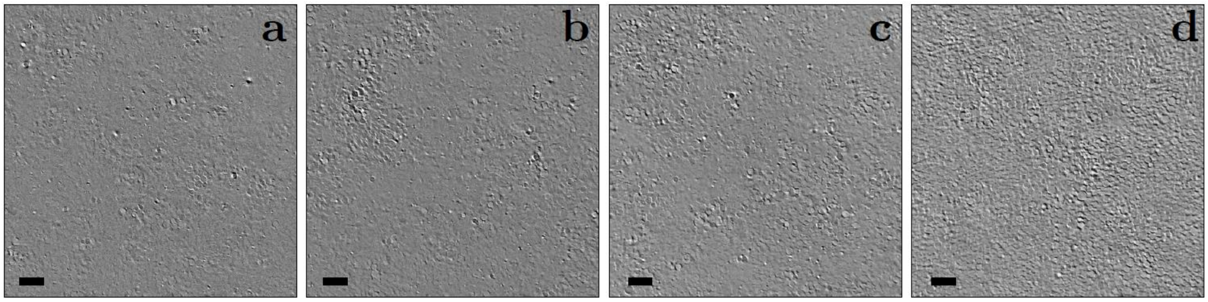


**Figure SI16: Coexistence of fast and slow domains as probed by microscopy**.

Images obtained by taking the intensity difference between two sample snapshots separated by time delays $\tau/T$ = 1 (a), 10 (b), 100 (c), 1000 (d). Data for sample E65%, in the coexistence region (strain amplitude $\gamma_0$ = 3.9%). Scale bar: 10 µm.

Finally, in simulations, we find that the system always segregates in mesoscopic domains similar to those shown in Fig. 3c of the main text, with no formation of macroscopic shear bands. An example for various imposed shear amplitudes spanning the coexistence region is shown in Fig. SI17.

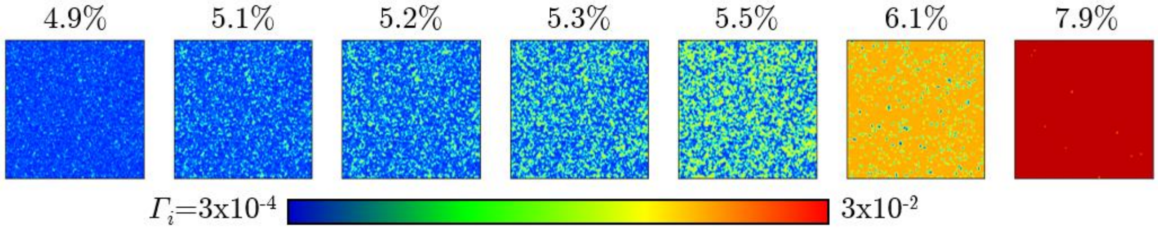


**Figure SI17: Coexistence of slow and fast relaxation rates at yielding.**

Snapshots of local normalized relaxation rates, $\Gamma_i$, at various applied strain amplitudes $\gamma_0$ indicated above each panel from lattice simulations. The model parameters are issued from the fit to sample N45% (see Table SI2). $\Gamma_i$ increases logarithmically from blue to red, as shown by the color bar. Each lattice is composed of 512 x 512 sites, with periodic boundary conditions along both directions.

## REFERENCES

[1] B. J. Berne and R. Pecora, *Dynamic Light Scattering: With Applications to Chemistry, Biology, and Physics* (Wiley, 1976).
[2] S. Aime, L. Ramos, J.M. Fromental, G. Prévot, R. Jelinek, and L. Cipelletti, *A stress-controlled shear cell for small-angle light scattering*, Rev. Sci. Instrum. **87**, 123907 (2016)
[3] E. D. Knowlton, private communication.
[4] F. Giavazzi and R. Cerbino, *Digital Fourier Microscopy for Soft Matter Dynamics*, Journal of Optics **16**, 083001 (2014).
